# Supplementary material for: Reservation of Virtualized Resources with Optimistic Online Learning
Source: arXiv:2303.08772 source file (2023-03-15)
Supplement: Supplementary file 1 [file appendix_G4.tex]

\section*{Appendix} 

We detail how we obtain the theoretical regret bound of the OOLRgrad solution.
First, we apply the ARMA-OGD on each gradient item and we obtain the regret bound for item $i$:
$$\sum_{t=1}^T (\grad_i f_t(\bm z_t) - \grad_i \tilde{f}_t(\bm \tilde{z}_t))^2 = Res + \mathcal{O}(GM\sqrt{T}),$$
where $Res$ is the residual error of the best ARMA prediction method with full hindsight, $G$ and $M$ are key constant in \cite{anava}.
Thus, we obtain the regret bound: $$\sum_{t=1}^T ||\grad f_t(\bm z_t) - \grad \tilde{f}_t(\bm \tilde{z}_t)||^2 = 2m Res + \mathcal{O}(2mGM\sqrt{T}).$$
Thus we rewrite the regret bound in \eqref{eq:regret_bound2} as:
$$R(T) = \mathcal{O}\Big(2D\sqrt{2T}\sqrt{2mRes+\mathcal{O}(2mGM\sqrt{T})}\Big).$$
Within the square root, we neglect $2mRes$ in front of $\mathcal{O}(2mGM\sqrt{T})$, hence we can simplify: $$R(T)=\mathcal{O}(4D\sqrt{mGM} T^{3/4}) = \mathcal{O}(T^{3/4}).$$
